# Supplementary material for: RPM-Net: Robust Point Matching using Learned Features
Source: arXiv:2003.13479 ancillary file (2020-03-30)
Supplement: Supplementary file 1 [file supplementary.pdf]

# RPM-Net: Robust Point Matching using Learned Features - Supplementary Material

Zi Jian Yew Gim Hee Lee
Department of Computer Science, National University of Singapore
{zijian.yew, gimhee.lee}@comp.nus.edu.sg

## 1. Chamfer Distance Metric

As explained in the main paper, our Chamfer distance metric is modified to consider the clean and complete version of the point clouds. In Figure 1, we show why this modification is necessary. As illustrated by the toy example, the original chamfer distance has the tendency to favor solutions where the point clouds are incorrectly "lumped" together when evaluating partial point cloud matching.

We also show in Figure 2 the rotation/translation errors and our modified Chamfer distance metric for several example alignments. Figure 2(a) shows a vase with a full rotational symmetry, and any solution rotated about its vertical axis is a plausible solution. Similarly, the partial visibility scenario sometimes also results in rotational symmetry, such as the staircase in Figure 2(b). However, such alternate solutions are penalized by the rotation error, as can be seen from the alignments in Figure 2(a) right and Figure 2(b) right having a 31.4° and 32.8° rotational errors despite being valid solutions. Our Chamfer distance metric does not penalize these alternate solutions and still gives a small error in both cases. On the other hand, it is more sensitive to certain misalignments than considering the translation or rotation error alone. Figure 2(c) and Figure 2(d) show clearly incorrect alignments which still result in small translation or rotation errors respectively. In both of these cases, the Chamfer metric gives a large error.

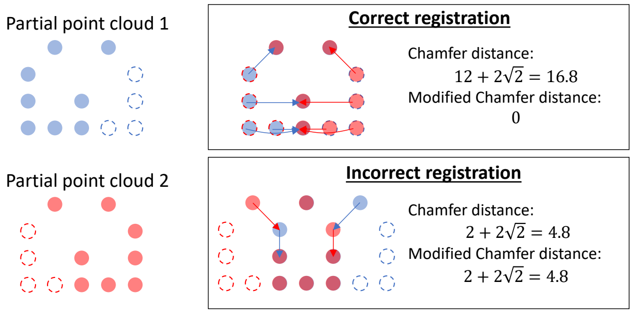


Figure 1. Chamfer distance metrics on a toy example. Arrows indicate vectors to nearest points. Unlike our modified metric, the original metric gives an erroneous lower error to the incorrect registration.

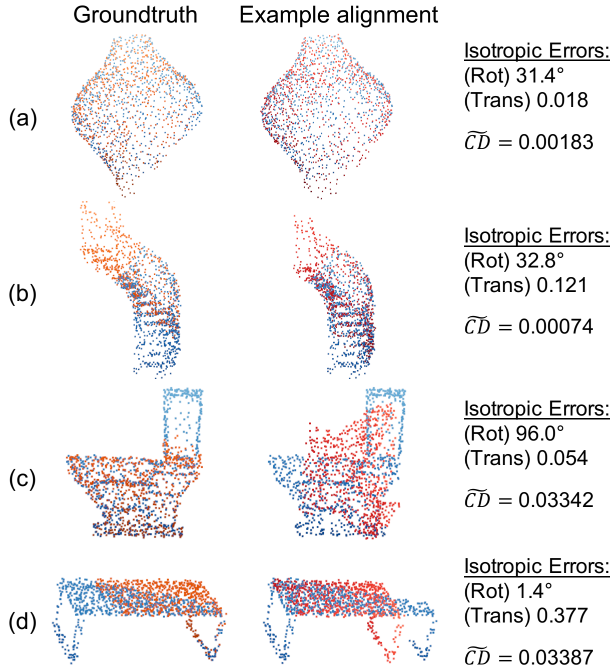


Figure 2. Example alignments and their error metrics

## 2. Predicted inliers

We visualize in Figure 3 the predicted inlier weights at each iteration for the source and reference point clouds, *i.e.* $w_j = \sum_k m_{jk}$ and $w_k = \sum_j m_{jk}$. The inlier weights in the first iteration are fairly arbitrary. However as the registration converges, the higher weights are assigned to the points within the overlapping region. This allows the network to reject and ignore points without correspondences.

### 2.1. Generalization to Real Data

We observe that our trained network is able to generalize to several real laser scans from the Stanford 3D Scanning

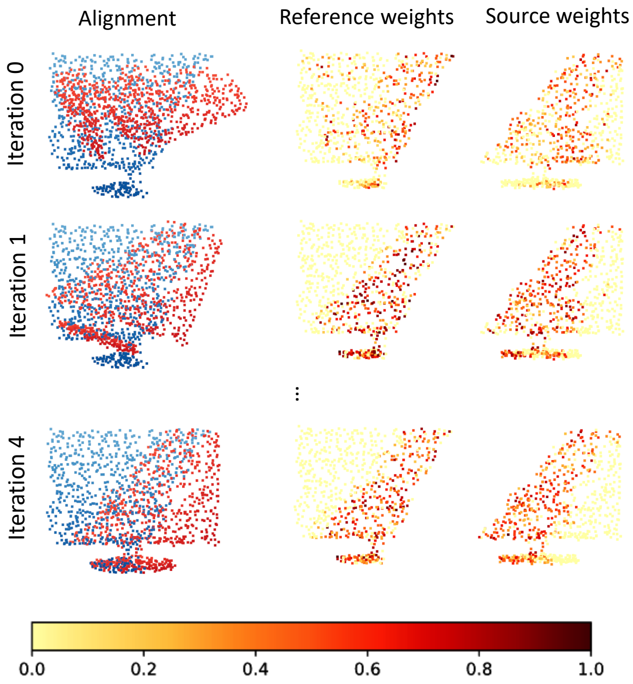


Figure 3. Predicted inlier weights at each iteration

Repository[1], despite not being trained on real world data. We preprocess the point clouds in the following manner to be consistent with the ModelNet40 data used in training: 1) uniform downsample by taking every $k^{\text{th}}$ point such that there is approximately 1024 points remaining, and 2) translate and scale the point clouds such that the point cloud fits approximately into a unit sphere. Figure 4 shows our registration results on two models of the dataset.

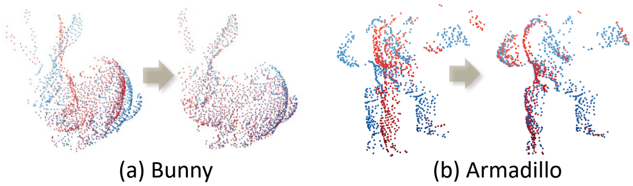


Figure 4. Registration of (a) Bunny and (b) Armadillo models from the Stanford 3D Scanning Repository. The Bunny and Armadillo models are acquired $45^\circ$ and $30^\circ$ apart respectively.

## 3. Additional Qualitative Results

Additional registration examples can be found on the project webpage[2].

[1] http://graphics.stanford.edu/data/3Dscanrep/
[2] https://github.com/yewzijian/RPMNet

## 4. Detailed Network Architecture

We show the detailed architectures of our Feature Extraction and Parameter Prediction networks in Tables 1 and 2, respectively. Both networks use a PointNet-based [1] architecture. We use the following notation: $N$ denotes the number of points in the point cloud, and $S$ denotes the number of points sampled in the neighborhood cluster for each point. Parameters for fully connected (FC) layers are given as (input-dim, output-dim), and the parameter for group normalization (GN) [2] is the number of groups used.

| Layer | Parameters | Output dimension |
|---|---|---|
| Shared FC | (10, 96) | $N \times S \times 96$ |
| GN + ReLU | (8) | $N \times S \times 96$ |
| Shared FC | (96, 96) | $N \times S \times 96$ |
| GN + ReLU | (8) | $N \times S \times 96$ |
| Shared FC | (96, 192) | $N \times S \times 192$ |
| GN + ReLU | (8) | $N \times S \times 192$ |
| Max pool | - | $N \times 192$ |
| FC | (192, 192) | $N \times 192$ |
| GN + ReLU | (8) | $N \times 192$ |
| FC | (192, 96) | $N \times 96$ |
| GN + ReLU | (8) | $N \times 96$ |
| FC | (96, 96) | $N \times 96$ |
| $\ell^2$ normalization | - | $N \times 96$ |

Table 1. Architecture of our Feature Extraction Network. It takes in $S \times 10$-dimensional raw features for each point cluster and outputs a 96-dimensional feature descriptor.

| Layer | Parameters | Output dimension |
|---|---|---|
| Shared FC | (4, 64) | $N \times 64$ |
| GN + ReLU | (8) | $N \times 64$ |
| Shared FC | (64, 64) | $N \times 64$ |
| GN + ReLU | (8) | $N \times 64$ |
| Shared FC | (64, 64) | $N \times 64$ |
| GN + ReLU | (8) | $N \times 64$ |
| Shared FC | (64, 128) | $N \times 128$ |
| GN + ReLU | (8) | $N \times 128$ |
| Shared FC | (128, 1024) | $N \times 1024$ |
| GN + ReLU | (16) | $N \times 1024$ |
| Max pool | - | 1024 |
| FC | (1024, 512) | 512 |
| GN + ReLU | (8) | 512 |
| FC | (512, 256) | 256 |
| GN + ReLU | (8) | 256 |
| FC | (256, 2) | 2 |
| Softplus activation | - | 2 |

Table 2. Architecture of our Parameter Prediction Network. The input is the spatial coordinates of the source and reference point clouds concatenated together, augmented with a 0 or 1 depending on which point cloud the point originates from. The network outputs the 2 parameters $\alpha, \beta$ used in the annealing.

## References


[1] Charles R. Qi, Hao Su, Kaichun Mo, and Leonidas J Guibas. Pointnet: Deep learning on point sets for 3D classification and segmentation. In *IEEE Conference on Computer Vision and Pattern Recognition (CVPR)*, pages 77–85, 2017. 2

[2] Yuxin Wu and Kaiming He. Group normalization. In *European Conference on Computer Vision (ECCV)*, pages 3–19. Springer, 2018. 2
